# Supplementary material for: Evidence of Antineutrinos from Distant Reactors using Pure Water at SNO+
Source: arXiv:2210.14154 source file (2023-03-28)
Supplement: Supplementary file 1 [file SNOplus_ReactorNuWater_Supplemental.pdf]

# SNO+ Experiment
## Supplemental Material
October 2022

This document provides supplemental information relevant to the evidence of reactor antineutrinos presented in the Letter "Evidence of Antineutrinos from Distant Reactors using Pure Water at SNO+".

## CONTENTS

I. Discovery Significance Formula 2

II. Event Information 2
II.1. Event distributions: LR method 3
II.2. Event distributions: BDT method 4

References 4

## I. DISCOVERY SIGNIFICANCE FORMULA

This Letter calculated a discovery significance of reactor $\overline{\nu}_e$using the formula derived in Ref. [1], which applies to counting experiments with uncertainties in backgrounds. The formula is

$$\left[2\left((s+b)\log\left[\frac{(s+b)(b+\sigma_b^2)}{b^2+(s+b)\sigma_b^2}\right]-\frac{b^2}{\sigma_b^2}\log\left[\frac{(s+b)\sigma_b^2+b^2}{b\sigma_b^2+b^2}\right]\right)\right]^{1/2}. \tag{1}$$

Substituting predicted values for $s$, $b$, and $\sigma_b^2$, provides the median discovery sensitivity. Substituting an observed value in place of $(s+b)$ provides the discovery significance.

In the limit of small $\sigma_b^2$ and small signal rate ($s << b$), this reduces to

$$\frac{s}{\sqrt{b+\sigma_b^2}}\left(1+O(s/b)+O(\sigma_b^2/b)\right). \tag{2}$$

If these conditions are not satisfied, this limiting expression greatly overestimates the significance.

## II. EVENT INFORMATION

Table I provides information about every event selected by the LR and BDT methods. Figures 1 and 2 show the distribution of selected events in the LR and BDT methods respectively.

TABLE I. Information about the 14 prompt-delayed coincidence pairs selected by the LR and BDT methods. Events not within the fiducial volume for the LR analysis are marked with '-' in the corresponding column. Nhits is the number of PMTs that detected a photon, $E$ is the reconstructed energy, $\rho \equiv \sqrt{x^2+y^2}$ is the transverse position, $z$ is the vertical position, $\mathbf{u}\cdot\mathbf{r}$ is the radial direction cosine, $\beta_{14}$ quantifies the isotropy of hit PMTs, $\Delta t$ is the time between prompt and delayed events, $\Delta r$ is the distance between prompt and delayed events, LR is the likelihood ratio value, and PBDT and DBDT are the prompt and delayed BDT values. See the Letter for more details about these variables. The three pairs without an LR value did not satisfy the initial fiducial volume selections and therefore were not accessible to the PDFs.

| Prompt | | | | | | Delayed | | | | | | | | | | |
|---|---|---|---|---|---|---|---|---|---|---|---|---|---|---|---|---|
| Nhits | $E$ [MeV] | $\rho$ [m] | $z$ [m] | $\mathbf{u}\cdot\mathbf{r}$ | $\beta_{14}$ | Nhits | $E$ [MeV] | $\rho$ [m] | $z$ [m] | $\mathbf{u}\cdot\mathbf{r}$ | $\Delta t$ [$\mu$s] | $\Delta r$ [cm] | LR | PBDT | DBDT | Date |
| 22 | 3.3 | 3.2 | -3.2 | 0.29 | -0.08 | 11 | 2.0 | 4.0 | -2.1 | 0.45 | 47 | 145 | 5.9 | 0.27 | 0.30 | 2018/11/29 |
| 35 | 4.8 | 6.9 | -1.3 | -0.2 | 0.42 | 10 | 1.8 | 6.1 | -1.2 | 0.89 | 66 | 112 | 10.5 | 0.20 | 0.22 | 2018/12/11 |
| 33 | 4.3 | 4.4 | -0.6 | -0.01 | 0.44 | 13 | 2.5 | 4.8 | 0.5 | -0.96 | 438 | 143 | 9.1 | 0.49 | 0.10 | 2018/12/24 |
| 24 | 4.1 | 5.5 | 3.5 | 0.66 | 0.61 | 10 | 2.4 | 4.9 | 4.3 | 0.68 | 136 | 103 | 11.0 | 0.39 | 0.30 | 2018/12/30 |
| 32 | 5.0 | 1.9 | -4.0 | 0.13 | 0.48 | 13 | 2.3 | 1.3 | -4.5 | 0.37 | 149 | 79 | 14.0 | 0.50 | 0.31 | 2019/01/20 |
| 36 | 4.6 | 4.2 | -0.2 | 0.43 | 0.57 | 10 | 1.6 | 5.0 | 0.0 | -0.64 | 177 | 90 | 9.6 | 0.57 | 0.05 | 2019/02/07 |
| 25 | 3.7 | 4.4 | -1.3 | 0.10 | 0.48 | 15 | 2.2 | 4.0 | -1.2 | -0.67 | 292 | 86 | 8.6 | 0.38 | 0.21 | 2019/02/15 |
| 26 | 4.2 | 5.2 | -1.4 | 0.19 | 0.35 | 11 | 2.4 | 5.5 | -1.6 | 0.68 | 115 | 45 | NA | 0.43 | 0.46 | 2019/03/04 |
| 38 | 5.6 | 4.1 | 3.6 | 0.71 | 0.35 | 10 | 2.5 | 4.4 | 4.2 | 0.68 | 346 | 68 | NA | 0.58 | 0.31 | 2019/03/06 |
| 22 | 3.8 | 5.0 | -2.3 | -0.31 | 0.62 | 11 | 1.8 | 5.0 | -2.5 | 0.83 | 165 | 19 | 9.5 | 0.27 | 0.40 | 2019/03/11 |
| 40 | 6.2 | 4.4 | -1.5 | 0.38 | 0.68 | 13 | 2.3 | 3.7 | -2.6 | -0.012 | 43 | 137 | 11.5 | 0.66 | 0.39 | 2019/03/22 |
| 25 | 3.6 | 3.8 | -3.5 | -0.40 | 0.24 | 10 | 1.9 | 4.5 | -3.6 | 0.67 | 265 | 83 | NA | 0.24 | 0.24 | 2019/05/02 |
| 23 | 3.7 | 2.4 | 3.1 | -0.31 | 0.41 | 11 | 1.9 | 1.3 | 2.6 | 0.39 | 196 | 195 | 6.6 | 0.39 | 0.28 | 2019/05/18 |
| 36 | 4.9 | 6.1 | -2.9 | -0.53 | 0.14 | 16 | 2.4 | 6.1 | -2.9 | 0.19 | 183 | 29 | 12.5 | 0.20 | 0.29 | 2019/07/09 |

### II.1. Event distributions: LR method

FIG. 1. Distributions for the events selected by the LR method. In (a) - (e) the background components are normalized to their expected counts, while the IBD signal is normalized to the total number of observed events minus the total number of expected background events. In (f) the signal (red) is normalized to the expectation. In (g) the dashed lines represent the fiducial boundaries around the AV.

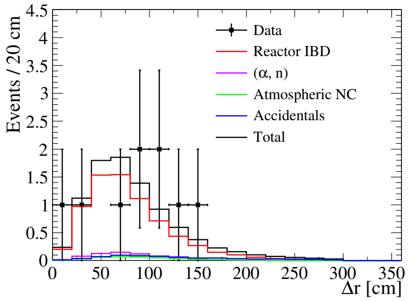


(a) Distance between events

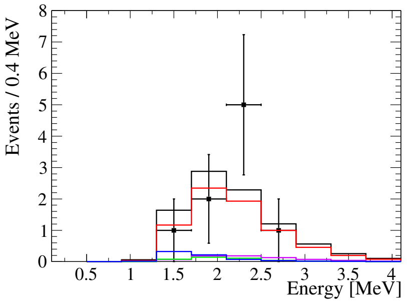


(b) Delayed events

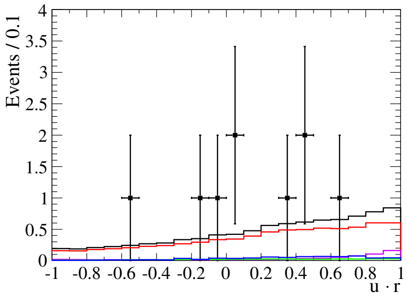


(c) Prompt events

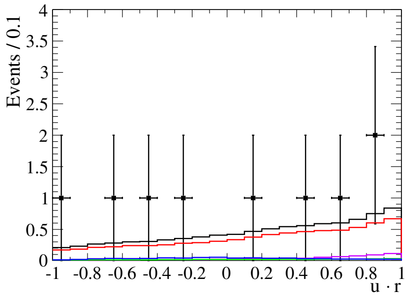


(d) Delayed events

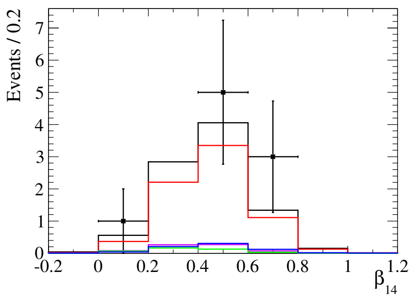


(e) Prompt events

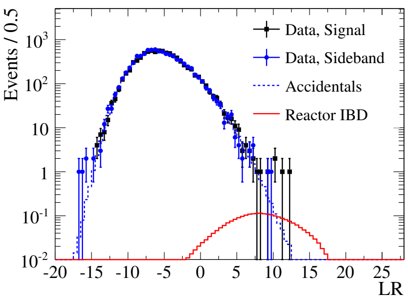


(f) External events

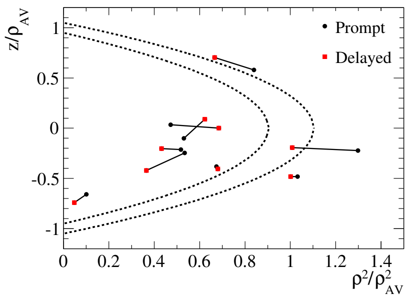


(g) Spatial distribution

## II.2. Event distributions: BDT method

FIG. 2. Distributions for the events selected by the BDT method. In (a) - (f) the background components are normalized to their expected counts, while the IBD signal is normalized to the total number of observed events minus the total number of expected background events. In (g) the dashed lines represent the fiducial boundaries around the AV.

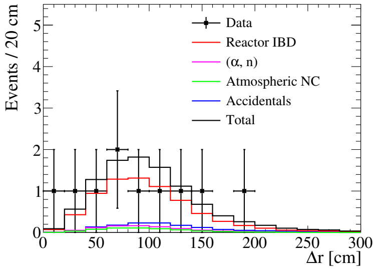


(a) Distance between events

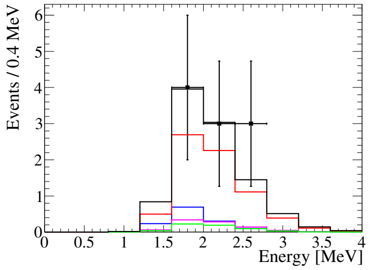


(b) Delayed events

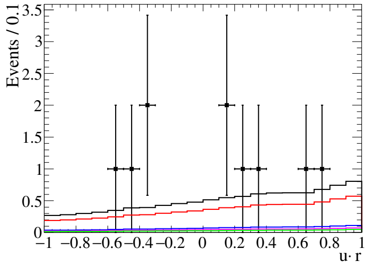


(c) Prompt events

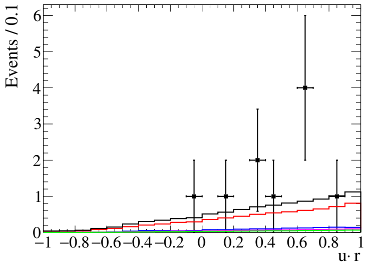


(d) Delayed events

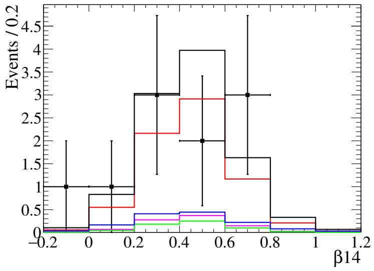


(e) Prompt events

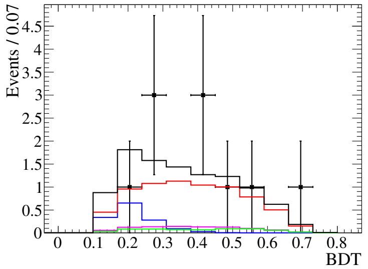


(f) Prompt events

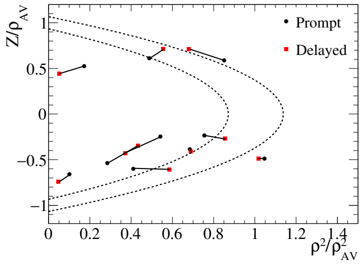


(g) Spatial distribution

[1] G. Cowan, Discovery sensitivity for a counting experiment with background uncertainty, https://www.pp.rhul.ac.uk/~cowan/stat/medsig/medsigNote.pdf (2012), last accessed in April 2022.
